# Supplementary material for: Sparse Projection Oblique Randomer Forests
Source: arXiv:1506.03410 source file (2019-10-03)
Supplement: Supplementary file 1 [file Appendix.tex]

% \renewcommand{\thesection}{A}
% \renewcommand{\thesubsection}{A.\arabic{subsection}}
% \section{Appendix}

\appendices

\clearpage

\onecolumn

\section{Pseudocode}

\input{pseudocodes.tex}

% \clearpage
\twocolumn

\section{Existing Decision Forest Algorithms as Special Cases of RerFs}
Most of the previously proposed decision forest algorithms sample a candidate set of randomly oriented split directions and choose the best one. They mainly differ in the probability distribution over the split directions. Hence, they are all different special cases of RerFs. Table \ref{table:algs} summarizes various algorithms within the RerF framework. 

\input{algorithm_table.tex}

\section{Random Vectors in High Dimensions}
\label{section: vectors}

A previous study demonstrated that a particular setting of F-RC that samples split projections with a fixed sparsity of $2/p$ significantly outperforms a method called Random Rotation Random Forest \cite{Blaser2016,Tomita2017}. Both can be viewed as particular special cases of the RerF framework, with the former sampling a sparse rectangular matrix $\mathbf{A} \in \Real{R}^{d \times p}$ and the latter sampling a dense square rotation matrix $\mathbf{A} \in SO(d)$. Here we provide geometric intuition which may serve as a possible explanation for these results, thereby motivating the adoption of sparse random projections for sampling splits, rather than dense random rotation matrices. Let $v^*$ be a hypothetical locally optimal split projection in $p$ dimensions at a generic split node. We sample $\mathbf{A}$ according to a specified distribution $f_\mathbf{A}$ and measure the angle of the closest univariate projection in $\mathbf{A}$. If we repeat this many times, we can estimate the probability of sampling a projection whose direction comes within some angle $\Theta$ of $v^*$. We performed this experiment using both the $f_\mathbf{A}$ adopted by the default implementation of RerF and that adopted by RR-RF, which is simply a rotation matrix. For RerF, two values of $d$, which specifies the number of columns in $\mathbf{A}$, were tested. Note for RR-RF that since $\mathbf{A}$ is a rotation matrix, it will always be $p \times p$. Two cases were tested for $v^*$. In one case, $v^*$ has a single nonzero. That is, the split is sparse. In another case, $v^*$ is all ones (dense). We repeated this experiment 10000 times for various values of $p$. Figure \ref{fig:intuition2} shows that when $v^*$ is sparse, RerF has a high probability of sampling a projection close in angle to $v^*$ for all values of $p$, while RR-RF has a low probability of sampling a close projection. On the other hand, when $v^*$ is dense and $p$ is large, both RerF and RR-RF have a very low probability of sampling a projection close in angle to $v^*$. These results are in line with established theory on high-dimensional random vectors, which says that as the number of dimensions increases, the probability that two random vectors are nearly orthogonal tends to one \cite{Vershynin2017}.
% @tt: we never refer to this in the main paper.  if we don't have a reference to it, we should remove it. i don't feel strongly about including it or not.

\begin{figure}[h!]
\vskip 0.2in
\begin{center}
\centerline{\includegraphics[width=\columnwidth]{vector_angle_probability.pdf}}
\caption{The probability that RerF and RR-RF sample a projection within an angle $\theta$ of some hypothetical optimal node projection $v^*$ in $p$ dimensions when the density (number of nonzeros) $\lambda^*$ of $v^*$ is minimal ($\lambda^* = 1/p$) and when it is maximal ($\lambda^* = 1$) for varying values of $\theta$ and $p$. When the optimal projection is sparse (A - D), RerF has a reasonable probability of sampling projections close to it for all values of $p$. The probability of RR-RF sampling a close projection quickly degrades with increasing $p$. When the optimal projection is dense (E - H), both RerF and RR-RF have a low probability of sampling a close projection for $p \geq 16$. Therefore, when the number of dimensions is large, it may be safer to assume $v^*$ is sparse and use a sampling distribution such as that adopted by RerF rather than the one adopted by RR-RF.}
\label{fig:intuition2}
\end{center}
\vskip -0.2in
\end{figure}

\section{Synthetic Datasets}
\label{section: synth_data}

\textbf{Sparse Parity} is a  multivariate generalization of the noisy XOR problem. It is a $p$-dimensional two-class problem in which the class label is $0$ if the number of dimensions having positive values amongst the first $p^* < p$ dimensions is even and $1$ otherwise. Thus, only the first $p^*$ dimensions carry information about the class label, and no individual dimension contains any information. Specifically, let $X = (X_1,\ldots,X_p)$ be a $p$-dimensional feature vector, where each $X_1,\ldots,X_p \overset{iid}{\sim} U(-1,1)$. Furthermore, let $S = \sum_{j=1}^{p^*}{\mathbb{I}(X_j>0)}$, where $p^* < p$ and $\mathbb{I}(X_j > 0)$ is the indicator that the $jth$ feature of a sample point $x$ has a value greater than zero. A sample's class label $Y$ is equal to the parity of $S$. That is, $Y = odd(S)$, where $odd$ returns 1 if its argument is odd and 0 otherwise. The Bayes optimal decision boundary for this problem is a union of hyperplanes aligned along the first $p^*$ dimensions. For the experiments presented in the following sections, $p^* = 3$ and $p = 20$. Figure~\ref{fig:error_synthetic} (A,B) show cross-sections of the first two dimensions taken at two different locations along the third dimension.

\textbf{Orthant} is a multi-class problem in which the class label is determined by the orthant in which a datapoint resides. A key characteristic of this problem is that the individual dimensions are strongly and equally informative. An orthant in $\Real^p$ is a generalization of a quadrant in $\Real^2$. In other words, it is a subset of $\Real^p$ defined by constraining each of the $p$ coordinates to be positive or negative. For instance, in $\Real^2$, there are four such subsets: $(X_1, X_2)$ can either be in 1) $\Real^+\times \Real^+$, 2) $\Real^- \times \Real^+$, 3) $\Real^- \times \Real^-$, or 4) $\Real^+ \times \Real^-$ . Note that the number of orthants in $p$ dimensions is $2^p$. Specifically for our experiments, we sample each $X_1,\ldots,X_p \overset{iid}{\sim} U(-1,1)$. Associate a unique integer index from $1$ to $2^p$ with each orthant, and let $O(X)$ be the index of the orthant in which $X$ resides. The class label is $Y = O(X)$. The Bayes optimal decision boundary in this setting is a union of hyperplanes aligned along each of the $p$ dimensions. We set $p = 6$ in the following experiments. Figure \ref{fig:error_synthetic} (D,E) show cross-sections of the first two dimensions taken at two different locations along the third dimension.

\textbf{Trunk} is a balanced two-class problem in which each class is distributed as a $p$-dimensional multivariate Gaussian with identity covariance matrices \cite{Trunk1979}. Every dimension is informative, but each subsequent dimension is less informative than the last. The means of class 1 and 0 are $\mu_1 = (1,\frac{1}{\sqrt{2}},\frac{1}{\sqrt{3}},...,\frac{1}{\sqrt{p}})$ and $\mu_0 = -\mu_1$, respectively. The Bayes optimal decision boundary is the hyperplane $(\mu_1 - \mu_0) \cdot X = 0$. We set $p = 10$ in the following experiments.

\section{Dataset Preprocessing}
\label{section: preprocess}

The classifiers were evaluated on 105 classification benchmark datasets derived from the UCI Machine Learning Repository. The following preprocessing steps were carried out, in the order listed, prior to classifier evaluation:

\begin{enumerate}
\item \textbf{Removal of nonsensical features}. Some features, such as unique sample identifiers, or features that were the same value for every sample, were removed.
\item \textbf{Imputation of missing values}. The R randomForest package was used to impute missing values. This method was chosen because it is nonparametric and is one of the few imputation methods that can natively impute missing categorical entries.
\item \textbf{One-hot-encoding categorical features}. Most classifiers cannot handle categorical data natively.
% @tt: define one - hot encoding
\item \textbf{Integer encoding of ordinal features}. Categorical features having order to them, such as "cold", "luke-warm", and "hot", were numerically encoded to respect this ordering with integers starting from 1.
\item \textbf{Standardization of the format}. Lastly, all datasets were stored as CSV files, with rows representing observations and columns representing features. The class labels were placed as the last column.
\item \textbf{Five-fold paritioning}. Each dataset was randomly divided into five partitions for five-fold cross validation. Partitions preserved the relative class frequencies as much as possible.
\end{enumerate}

\section{Hyperparameter Tuning}
\label{section: tuning_app}

Hyperparameters in XGBoost are tuned via grid search using the R caret package. The values tried for each hyperparameter are based on suggestions by Owen Zhang (\url{https://www.slideshare.net/OwenZhang2/tips-for-data-science-competitions}), a research data scientist who has had many successes in data science competitions using XGBoost:
% @jy: i might compress "itemize" too. or change this to a list, rather than it getting its own display environment.
% from jy: Echoing your comment from below, I think this should also be in the appendix. 
\begin{itemize}
\item nrounds: 100, 1000
\item subsample: 0.5, 0.75, 1 
\item eta: 0.001, 0.01
\item colsample\_bytree: 0.4, 0.6, 0.8, 1
\item min\_child\_weight: 1
\item max\_depth:~4, 6, 8, 10, 100000
\item gamma: 0
\end{itemize}

Selection of the hyperparameter values is based on minimization of a five-fold cross-validation error rate.

% \section{Benchmark Results}\label{section: error_table}

% @tt: your table is a bit cut-off.  maybe make the font "tiny".  alternately, make sure the number of significant digits  \geq floor(1/n).  i'd also left justify all the numbers, it is hard to read with so many implicit vertical lines.
% \input{benchmark_error_table2.tex} 

\section{Theorem Proofs}\label{section: pfs}

\section{Bayes Error of Trunk's Problem Along a Univariate Projection}\label{section: bayes}
Suppose the prototypical pair $(X,Y) \in \Real^p \times \{c_1,\ldots,c_K\}$ has joint distribution $f_{XY}$. Let $L^*$ be defined as in Section \ref{section: consistency}, and $a \in \Real^p$ be a projection vector. Then the projection $X' = \, \langle X,a\rangle \, \in \Real$ of $X$ onto $a$ induces a joint distribution $f_{X'Y}$. The Bayes error with respect to $f_{X'Y}$ is denoted by $L'^*$.

In Trunk's problem, the task is to discriminate between two p-dimensional normal populations $N(\mu_0, \Sigma)$ and $N(\mu_1, \Sigma)$, where an observation comes from each population with equal probability and $\mu_0$, $\mu_1$ and $\Sigma$ are described as in Appendix \ref{section: synth_data}. The Bayes error for this problem is
\begin{align*}
L^* &= 1 - \Phi(\frac{1}{2}(\Delta^T\Sigma^{-1}\Delta)^{1/2}) \\
	&= 1 - \Phi(\frac{1}{2}||\Delta||_2) \\
    &= 1 - \Phi(||\mu_1||_2)
\end{align*}
where $\Phi$ is the standard normal cumulative distribution function and $\Delta = \mu_1 - \mu_0$ \cite{Bickel2004}. Now suppose we have an arbitrarily oriented projection vector $a$. Without loss of generality, let $||a||_2 = 1$. Using the fact that for Trunk's problem, any vector projection of $X$ is a sum of (scaled) independent random variables, it is straightforward to show that the Bayes error of $f_{X'Y}$ is
\begin{align*}
L'^* = 1 - \Phi(|\langle\mu_1,a\rangle|).
\end{align*}
